# Supplementary material for: Magnetically Confined Mountains on Accreting Neutron Stars in General Relativity
Source: arXiv:2309.09519 source file (2023-09-18)
Supplement: Supplementary file 1 [file appendixA.tex]

In this appendix, we remind the reader briefly about some basic properties of differential forms and exterior calculus. We do this with the aim of simplifying some tensorial equations in the theoretical framework presented in Section \ref{sec:GRMHD}, and to show how symmetry conditions are naturally represented in this framework. Symmetries are discussed further in Appendix \ref{app:sym}. We note that the results following from the exterior calculus can be derived equivalently by other, less formal methods (\cite{misner2017Gravitation}); they are noted here for completeness.

\subsection{Definitions}

A differential $p$-form is a completely antisymmetric tensor of type $(0,p)$. We also regard functions as $0$-forms and covectors as $1$-forms. We then define a product between forms called the \textit{wedge product}, denoted by $\wedge$, as
\begin{equation}
    \label{wedge_product}
    \paren{\go\wedge\alpha}_{a_{1}...a_{p}b_{1}...b_{q}}=
    \frac{(p+q)!}{p!q!}\go_{[a_{1}...a_{p}}\alpha_{b_{1}...b_{q}]}.
\end{equation}

\noindent The symbol $[]$ denotes the antisymmetrization operator. The wedge product of two differential forms is, again, a form. In particular, the product of two $1$-forms is
\begin{equation}
    \paren{\go\wedge\alpha}_{ab}=
    \go_{a}\alpha_{b}-\go_b\alpha_a.
\end{equation}

Another operation one can perform on forms is the \textit{Hodge dual}. For a $p$-form in a $n$-dimensional space, this is defined as
\begin{equation}
    \label{hodge_star}
    (\star\go)_{a_{1}...a_{n-p}}=\frac{1}{p!}\levidduu{a_{1}...a_{n-p}}{b_{1}...b_{p}}\go_{b_{1}...b_{p}},
\end{equation}

\noindent where $\epsilon$ is the totally antisymmetric tensor. Applying this definition to a $2$-form $F$ in a $4$-dimensional space, we have
\begin{equation}
    (\star F)_{ab}=\frac{1}{2}\levidduu{ab}{cd}F_{cd}.
\end{equation}
Finally, the \textit{exterior derivative} of a differential form is
\begin{equation}
	\label{exterior_dv}
	(\dd{\go})_{a_{1}...a_{p+1}} = (p+1)\codv{[a_1}{\go}_{a_{2}...a_{p}]},
\end{equation}
where $\nabla_a$ is any derivative operator on the manifold.

\subsection{Poincaré's Lemma}

An important result in the theory of differential forms is Poincaré's Lemma. This lemma, physically, associates tensorial quantities with their potential. Furthermore, it states under what conditions relevant physical quantities have an associated potential. We see in appendix \ref{app:sym} that due to the symmetries we assume for magnetically confined mountains, we can express all the magnetic quantities in terms of one scalar potential function $\psi$.

Definition \eqref{exterior_dv} immediately implies that $\dd(\dd\go)=0$ for any differential form $\go$, since the commutator of second derivatives of functions is zero. The converse question is whether an arbitrary p-form that satisfies $\dd\go=0$ can be written as $\go=\dd A$, for a certain choice of a $(p-1)$-form A. This question is answered by Poincaré's Lemma:

Let $F$ be a differential p-form such that $\dd F=0$. For a region of space without any singularities\footnote{For a rigorous approach, see \cite{carmo1998differential}.}, there exists a $(p-1)$-form $A$ such that
\begin{equation}
    \label{poin_lemma}
    F=\dd A.
\end{equation}
