# Supplementary material for: Magnetically Confined Mountains on Accreting Neutron Stars in General Relativity
Source: arXiv:2309.09519 source file (2023-09-18)
Supplement: Supplementary file 2 [file appendixC.tex]

Caution should be exercised when comparing Newtonian and general relativistic results. In Section \ref{sec:results}, we make several direct comparisons between the results in this paper and those by \cite{pm04}. This is done so one can see the differences that are introduced when considering relativity and how relevant they are. Nevertheless, a comparison such as this is ultimately artificial since the physical nature of the universe is relativistic and one can not simply `turn on' or `turn off' its effects; the Newtonian analysis is simply an approximation of reality. In practice, this raises challenges when choosing some parameters and variables for the governing equations. We highlight some of these problems in this appendix.

One challenge concerns the mass density variable $\rho$. In Newtonian mechanics, this quantity has a single definition. In general relativity, there are different variables that `play the role' of the Newtonian $\rho$. We can see this in the equation of state \eqref{isot_eos}; disturbances in a relativistic fluid propagate with velocity given by $c_s^2=\partial{p}/\partial{e}$, where $e$ is the energy density. That is, $e$ substitutes for the Newtonian $\rho$. In a different scenario, when we introduce the flux-freezing condition in Section  \ref{sec:flux-freezing}, we used the rest-mass density $\rho$ in equation \eqref{mass-flux}. This is due to the fact we prevent fluid elements from crossing between the level surfaces of $\psi$.

Comparing Newtonian and relativistic theory is also complicated when discussing electromagnetic effects. Equation \eqref{B_from_F} shows that the magnetic field is dependent on the observer who measures it, and equation \eqref{rad_dip_gr} shows that the form of the dipole is not the same in both theories. This leads to subtleties in setting the value of $\psi_*$ in our simulations. A way to approach this would be to fix a fiducial value of the polar magnetic field measured by a local observer in both theories and then compute the appropriate value of $\psi_*$. A second approach is to fix a fiducial value for $\psi_*$ and to use that value in both theories. The latter approach avoids the conversion of $B_*$ to $\psi_*$ and makes the simulations agree for the value of the dipole moment calculated with equation \eqref{dip_mom} at the surface. Given these helpful properties, we choose this approach. The results can be seen in Section \ref{sec:results}.
